# Supplementary material for: Logical Satisfiability of Counterfactuals for Faithful Explanations in NLI
Source: arXiv:2205.12469 source file (2022-05-25)
Supplement: Supplementary file 1 [file entailment_table_appendix.tex]

\begin{table}[!t]
%\small
\begin{tabular}{rrl}
\hline
Expl(Rel) & Hypothesis & Gold Label \\
\hline
\bm{$\neg (A \Leftrightarrow B)$} & \bm{$B$} & \textbf{Contradict} \\
$\neg (A \Leftrightarrow B)$ & $\tilde{B}$ & Contradict \\
$\neg (A \Leftrightarrow B)$ & $\neg B$ & Neutral \\

\hline
\hline
\bm{$ A \Leftrightarrow B$} & \bm{$B$} & \textbf{Entail} \\
$ \neg(A \Leftrightarrow B')$ & $B'$ & Contradict \\
$ \neg(A \Leftrightarrow \neg B
)$ & $\neg B$ & Contradict \\
$ A \Leftrightarrow B, B \Leftrightarrow \tilde{B}$ & $\tilde{B}$ & Entail \\

\hline
\hline 
\bm{$A \wedge \neg B$} & \bm{$B$} & \textbf{Neutral} \\
$A \wedge \neg B$ & $\tilde{B}$ & Neutral \\
$A \wedge \neg B$ & $\neg B$ & Neutral \\

\hline
\hline
Tautology & Hypothesis & Gold Label \\
\hline
\hline
$ A \Leftrightarrow A $ & $A$ & Entail \\
$ A \Leftrightarrow A, A \Leftrightarrow \tilde{A} $ & $\tilde{A}$ & Entail \\
$ \neg(A \Leftrightarrow \neg A) $ & $\neg A$ & Contradict/Neutral \\
$ \neg(A \Leftrightarrow A') $ & $A'$ & Contradict/Neutral \\

\end{tabular}
\caption{\small
[Placeholder entailment table - not everything will be used here, full table will go to appendix]
}
\suz{This is a data-augmentation table, not the one Anton wanted.}
%Entailment table for training with contrastive examples. The tautology examples can be constructed for every training data instance regardless of the label. For each gold label in bold, the additional training instances can be constructed based on the provided relation from the original explanation.}

\label{tab:hyp_results}
\end{table}
